# Supplementary material for: Time-Resolved Cavity Nano-Optomechanics in the 20-100 GHz range
Source: arXiv:1610.04179 source file (2016-10-13)
Supplement: Supplementary file 1 [file Supp_Material_Time-Resolved_Cavity_Nano-Optomechanics_SAnguiano.pdf]

# Supplementary Material: Time-Resolved Cavity Nano-Optomechanics in the 20-100 GHz range

S. Anguiano[1], A. E. Bruchhausen[1], B. Jusserand[2], I. Favero[3], F. R. Lamperti[3,4], Loic Lanco[4], I. Sagnes[4], A. Lemaître[4], N. D. Lanzillotti-Kimura[4], P. Senellart[4], and A. Fainstein[1,*]

[1]*Centro Atómico Bariloche & Instituto Balseiro, C.N.E.A., CONICET, 8400 S. C. de Bariloche, R. N., Argentina*

[2]*Institut des NanoSciences de Paris, UMR 7588 C.N.R.S. - Université Pierre et Marie Curie, 75015 Paris, France*

[3]*Université Paris Diderot, Sorbonne Paris Cité, Laboratoire Matériaux et Phénomènes Quantiques, CNRS-UMR 7162, 10 rue Alice Domon et Léonie Duquet, 75013 Paris, France and*

[4]*Centre de Nanosciences et de Nanotechnologies, C.N.R.S., Univ. Paris-Sud, Université Paris-Saclay, C2N Marcoussis, 91460 Marcoussis, France*

## Abstract

In this supplemental material we provide details of the experimental procedures used to determine mechanical mode lifetimes and amplitudes.

* email:afains@cab.cnea.gov.ar

## DETERMINATION OF MECHANICAL MODE LIFETIMES

We have used an ultrashort picosecond laser pump and probe reflectance difference set-up with micrometer size resolution to study the vibrational modes of the nano-optomecanichal resonators in the 20-100 GHz spectral range. For this technique both pump and probe need to be degenerate and resonant with the pillar cavity mode. To avoid "cross talking" of pump light into the detection channel both polarization and spatial filtering are required. Laser pulses of approximately 1 ps duration and repetition rate $f_r \sim 80$ MHz are separated into crossed polarized pump and probe beams with relative power controlled by a $\lambda/2$ retarder and a polarizing beam splitter. The pump beam is modulated at MHz frequencies to allow for phase sensitive detection. Both pump and probe pulses are then sent to imping on the pillar surface through the same microscope objective. An aperture is introduced before the latter as spatial filter to limit the back-reflected pump light collected by the same microscope and sent to the detector. Polarization filtering is attained by using first a polarizing beam splitter in the collection path, and then a second polarizer at the entrance to the detector.

The determination of the mechanical signal decay times is done as follows. We estimate the mechanical mode lifetime as $\tau = (t_2 - t_1)/ln(A_1/A_2)$, where $A_1(A_2)$ is the amplitude of the mechanical signal measured at delay time $t_1(t_2)$. Here the delay times is defined as $\Delta t = t_{probe} - t_{pump}$, with $t_{probe}(t_{pump})$ the arrival time of the probe(pump) pulse to the pillar. The method is more precise if both times, $t_1$ and $t_2$, are as separated as possible. The timing between pump and probe is set by passing the probe beam through a multi-pass 60 cm delay line. Six passes are required to cover the maximum accessible delay time attainable with our set-up, corresponding approximately to the 12.5 ns ($= f_r^{-1}$) separation between laser pulses. Because of the large distance covered by the delay-line, small focussing variations might occur for the larger displacements, which is a general concern of delay-line based set-ups. To comply with the condition of having $t_1$ and $t_2$ as separated as possible, and at the same time minimizing the effects of laser focussing, we chose to use as $t_2$ the mechanical mode amplitudes measured shortly *before* the pump-probe coincidence, that is, at *negative* delay times $\Delta t$. This signal is what remains from the previous pump pulse that impinged on the sample 12.5 ns before. In terms of the geometrical displacement of the delay line, this election of $t_2$ is the one that minimizes the geometrical separation corresponding to the two compared probe pulses.

The magnitude of the measured signal $A_1$ and $A_2$ is not only dependent on the amplitude of the coherent mechanical vibrations present in the device, but also on the transduction constant relating this vibrations to the induced change in reflectivity. This transduction constant depends on the detuning between the cavity mode and the laser wavelength. [1] For example, it is null for zero-detuning, and maximum when the cavity mode is tuned to the flanks where the derivative of the laser-mode's intensity profile is maximum. To take into account this situation, $t_1$ and $t_2$ need to be chosen so that the involved transduction constant is the same for the two cases. The smallest value that can be chosen for $t_1$, to minimize the focussing effects and avoid this transduction constant problem, corresponds to the time where the cavity mode has attained its equilibrium. This is signaled in the measured traces by the appearance of neat (not "chaotic") oscillations. This value is pillar size dependent, ranging for example from 1 ps to 4 ns for 3 $\mu$m and 10 $\mu$m pillars, respectively. To define the same values of $t_2$ for all cases we thus chose the larger value compatible with all, which correspond to 4.5 ns.

An example of the described procedure for the 5$\mu$m pillar is presented in Fig. S1. The error bars shown in Fig. 3 of the main text correspond to the uncertainty of the values of $A_1$ and $A_2$ obtained this way (oscillations of amplitude within the shaded squares), and to the variations observed by using other choices of $t_2$ (smaller values for example in Fig. S1). Within our experimental uncertainty we see no significant variation for the amplitudes at $t_1 = 12.5$ ns and $t_1 = 4.5$ ns for pillar sizes larger than 7 $\mu$m. We consequently assume $\tau \geq 20$ ns for these cases.

## LASER TO CAVITY-MODE OPTICAL COUPLING

The measured intensity of the observed mechanical signals depends naturally on the pump laser light intensity that effectively excites the pillars. In other words, in how many photons actually interact with the GaAs spacer (where the pump laser interaction occurs). This pump intensity depends, i) on the size of the laser spot that should match that of the pillar, and ii) on the spectral and numerical aperture matching between the laser and the optical cavity mode. The latter is illustrated by the shaded oval in Fig. 1(b) of the main text. In fact, both the mode angular distribution and spectral spread (Q-factor) depend on the pillar diameter. Keeping the focalization conditions constant, for large pillars a continuum

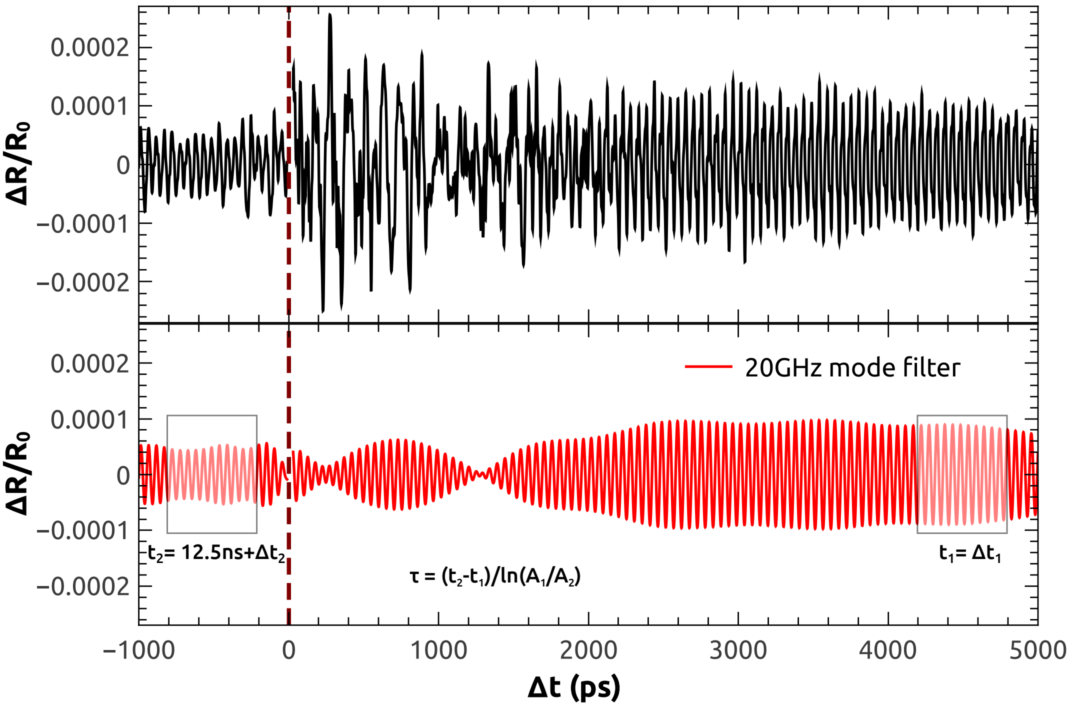


FIG. S1: **Procedure for the estimation of mechanical mode lifetimes.** The top panel shows the filtered differential reflectance time trace corresponding to the mechanical signal. The bottom panel shows the trace corresponding to the 20 GHz only. The shaded squares indicate the two delay times used to extract the mechanical mode lifetime $\tau = (t_2 - t_1)/ln(A_1/A_2)$, with $A_1(A_2)$ the mechanical signal amplitude measured at delay time $t_1(t_2)$.

of modes is excited, while for structures smaller than $\sim 8\mu$m only the fundamental cavity mode is accessed. When the pillar size is smaller than $\approx 5\mu$m, the angular spread of the cavity mode is indeed larger than that used in the focussing optics, meaning that the mode is underfilled. The focussing on the other hand is determined by the aperture used to limit the cross-talk between pump and probe pulses. All this limits the possibility to unambiguously determine the amount of pump light deposited in the sample. To avoid these potential issues we worked in a region of pump laser intensities that, due to the saturation of the coherent phonon generation process, are not strongly dependent on the deposited power.

To illustrate the procedure used, we show in Fig. S2 a color map representing the time-resolved evolution of the spectra of the probe light reflected from a 5 $\mu$m pillar. The curves have been normalized to the incident probe light intensity. The dark horizontal line

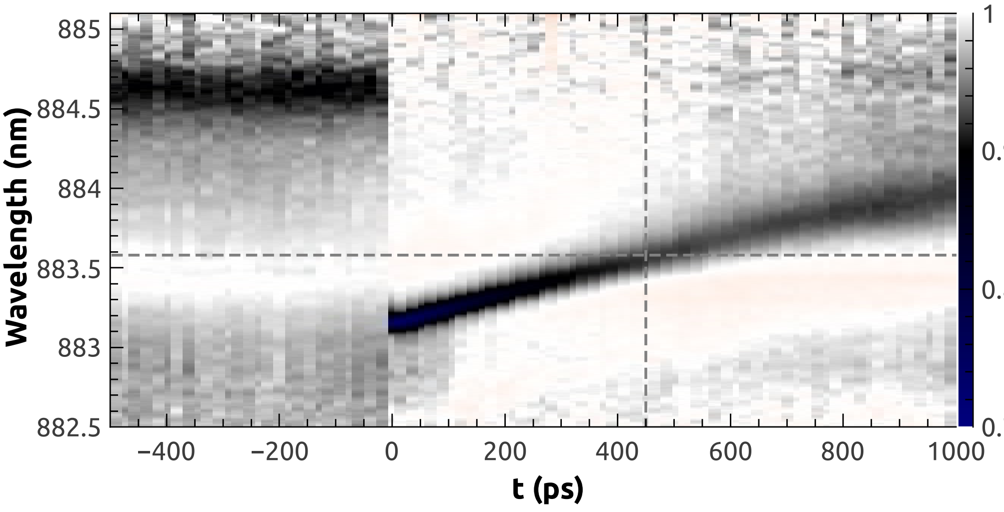


FIG. S2: **Time dependence of the pump induced optical cavity-mode shift.** The figure shows with a color map the time-resolved probe pulse reflectivity. The optical cavity mode observed at ≈ 884.6 nm at negative delay times blue-shifts up to ≈ 883.2 nm after the pulse excitation. The horizontal dashed line indicates the laser pulse central wavelength. The vertical dashed line corresponds to zero-detuning between laser pulse and optical cavity-mode.

observed at ≈ 884.6 nm at negative delay times corresponds to the unperturbed optical cavity-mode. Upon pump pulse excitation the mode rapidly shifts $\Delta\lambda \approx 1.4$ nm to ≈ 883.2 nm (and narrows). The horizontal dashed line in the figure indicates the laser pulse central wavelength. The laser FWHM is approximately 0.9 nm. The vertical dashed line corresponds to zero-detuning between laser pulse and optical cavity-mode.

We focus our attention here on the magnitude of the cavity-mode shift (maximum value at zero delay times), and on its relation to the mechanical signal amplitude. Both depend on the pump-laser power, as is illustrated in Fig. S3. It is quite clear from this figure that the two values are correlated, and also that there is a saturation which, for the shown pillar, occurs at powers $\simeq 5$ mW. Thus, even if for the different pillars the coupling conditions vary, we can assure that the signals will be independent of the deposited power if we are in the saturated regime.

Besides the pump power effects just described, the phonon induced variation of the reflected *probe* power will also naturally depend on the amount of light impinging on and reflected from the pillar's surface. In fact, the spatial aperture used in the experimental

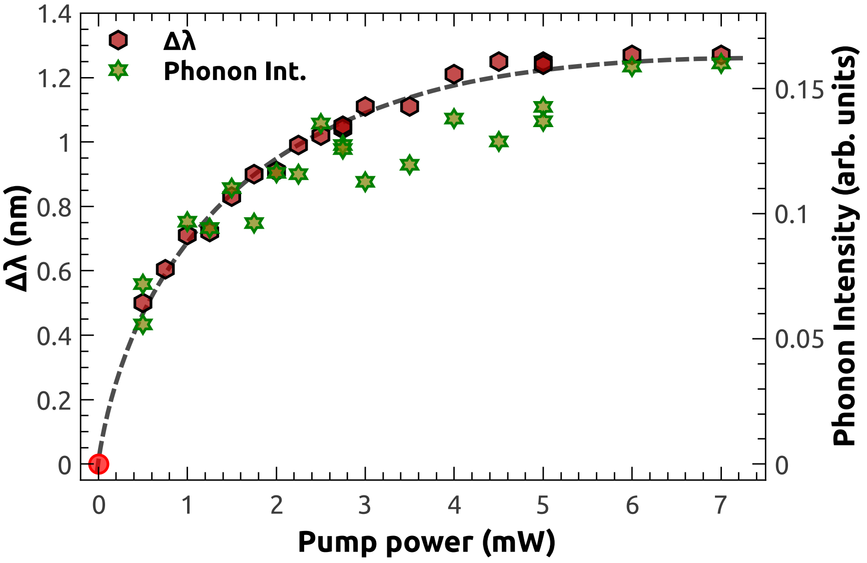


FIG. S3: **Pump power dependence.** Dependence of the 20 GHz mechanical signal amplitude (stars) and cavity-mode shift $\Delta\lambda$ (hexagons) with optical pump power. The red circle indicates the cavity-mode initial condition.

set-up limits the probe laser minimum spot size to values around $3-4\mu$m. This implies that for pillars of these sizes part of the light will be lost out of the pillar's top surface. To correct for this trivial effect we normalized the time-dependent phonon signals ($\Delta R$) with respect to the measured reflected continuous wave probe power ($R_0$).

One aspect that cannot be overlooked on analysing Fig. S1 is the fact that the mechanical mode lifetimes is longer than the 12.5 ns separation between the laser pulses. Thus, in principle the signal amplitude just described could be modified by the accumulation of excitations produced by successive laser pulses. One consequence of this would be that the signal amplitude could depend on the repetition rate, and more specifically could be resonant upon sub-harmonic driving, [2] complicating the comparison between different pillar sizes as done in Fig. 3 of the main text. To clarify this situation, we have done a study of the mechanical mode signal amplitude varying the repetition rate at values both far away from the sub-harmonic driving condition, and with high detail close to this condition. We have not observed any dependence of the observed mechanical signal on laser repetition rate. On one side, this has the direct implication that for small variation of micropillar mechanical frequencies we will be under similar coherent excitation conditions. Consequently we can

conclude that the comparison of signal amplitudes between different pillar sizes reported in Fig. 3 of the main text is reliable. One possible explanation for this lack of dependence on the repetition rate could be that the mechanical modes are so narrow (long lifetimes) that in the experiments we are never entering into a resonant driving regime. Another possibility would be that every pump produces such a strong alteration of the electronic landscape, and consequently of the equilibrium lattice position through deformation potential interaction, that all memories of existing vibrations are erased. The answer to these questions is currently being investigated.


[1] S. Anguiano, G. Rozas, A. E. Bruchhausen, A. Fainstein, B. Jusserand, P. Senellart, and A. Lemaître, Physical Review B **90**, 045314 (2014).

[2] A. Bruchhausen, R. Gebs, F. Hudert, D. Issenmann, G. Klatt, A. Bartels, O. Schecker, R. Waitz, A. Erbe, E. Scheer, J.-R. Huntzinger, A. Mlayah, and T. Dekorsy, Phys. Rev. Lett. **106**, 077401 (2011).
